# Supplementary material for: Thixotropic spectra and Ashby-style charts for thixotropy
Source: arXiv:2201.10004 ancillary file (2022-01-24)
Supplement: Supplementary file 1 [file SI.pdf]

# Thixotropic spectra and Ashby-style charts for thixotropy

Samya Sen, Randy H. Ewoldt
Department of Mechanical Science and Engineering
University of Illinois at Urbana-Champaign, Urbana, IL 61801, USA

## Supplementary Information

## 1 Probability density function for the stretched exponential function

It is possible to express a stretched exponential relaxation as a continuous sum of exponential decays [1, 2]

$$e^{-(t/\tau_{\mathrm{se}})^{\beta}} = \int_0^{\infty} \mathcal{H}\left(\xi; \tau_{\mathrm{se}}, \beta\right) e^{-\xi t} \mathrm{d}\xi, \tag{1}$$

where $\xi$ is a domain of rate constants. The underlying distribution is given by [1]

$$\mathcal{H}\left(\xi; \tau_{\mathrm{se}}, \beta\right) = \frac{1}{\pi}\tau_{\mathrm{se}} \int_0^{\infty} e^{-u^{\beta}\cos(\pi\beta/2)} \cos\left[\xi\tau_{\mathrm{se}}u - u^{\beta}\sin\left(\frac{\pi\beta}{2}\right)\right] \mathrm{d}u. \tag{2}$$

The stretched exponential relaxation can also be written as a distribution over a domain of time constants $\tau$ as [1]

$$e^{-(t/\tau_{\mathrm{se}})^{\beta}} = \int_0^{\infty} \mathcal{F}\left(\tau; \tau_{\mathrm{se}}, \beta\right) e^{-t/\tau} \mathrm{d}\tau, \tag{3}$$

where $\mathcal{F}$ is related to $\mathcal{H}$ through [1]

$$\mathcal{F}\left(\tau; \tau_{\mathrm{se}}, \beta\right) = \frac{1}{\tau^2}\mathcal{H}\left(\frac{1}{\tau}; \tau_{\mathrm{se}}, \beta\right). \tag{4}$$

The underlying distribution for the stretched exponential is thus

$$\mathcal{F}(\tau; \tau_{\mathrm{se}}, \beta) = \frac{1}{\pi}\frac{\tau_{\mathrm{se}}}{\tau^2} \int_0^{\infty} e^{-u^{\beta}\cos(\pi\beta/2)} \cos\left[\frac{\tau_{\mathrm{se}}}{\tau}u - u^{\beta}\sin\left(\frac{\pi\beta}{2}\right)\right] \mathrm{d}u. \tag{5}$$

To obtain the continuous spectrum for step shear data, consider step down tests as an example. The fit equation used is

$$\sigma^{+}(t) = \sigma_0 + \sigma_{\mathrm{se}}^{+}\left[1 - e^{-(t/\tau_{\mathrm{se}}^{+})^{\beta}}\right], \tag{6}$$

which can be written as a continuous spectrum as

$$\sigma^+(t) = \sigma_0 + \int_0^\infty X^+(\tau^+)\left(1 - e^{-t/\tau^+}\right) \mathrm{d}\tau^+. \tag{7}$$

Equating 6 and 7, we get

$$\sigma^+_{\text{se}}\left[1 - e^{-(t/\tau^+_{\text{se}})^\beta}\right] = \int_0^\infty X^+(\tau^+)\left(1 - e^{-t/\tau^+}\right) \mathrm{d}\tau^+. \tag{8}$$

From Eq. 3, we get

$$\sigma^+_{\text{se}}\left[1 - \int_0^\infty \mathcal{F}\left(\tau^+; \tau^+_{\text{se}}, \beta\right) e^{-t/\tau^+} \mathrm{d}\tau^+\right] = \int_0^\infty X^+(\tau^+)\left(1 - e^{-t/\tau^+}\right) \mathrm{d}\tau^+, \tag{9a}$$

$$\implies \sigma^+_{\text{se}} - \sigma^+_{\text{se}}\int_0^\infty \mathcal{F}\left(\tau^+; \tau^+_{\text{se}}, \beta\right) e^{-t/\tau^+} \mathrm{d}\tau^+ = \int_0^\infty X^+(\tau^+)\mathrm{d}\tau^+ - \int_0^\infty X^+(\tau^+)e^{-t/\tau^+} \mathrm{d}\tau^+, \tag{9b}$$

and this integral equation is valid iff both

$$\sigma^+_{\text{se}} = \int_0^\infty X^+(\tau^+)\mathrm{d}\tau^+, \tag{10}$$

and

$$\sigma^+_{\text{se}}\int_0^\infty \mathcal{F}\left(\tau^+; \tau^+_{\text{se}}, \beta\right) e^{-t/\tau^+} \mathrm{d}\tau^+ = \int_0^\infty X^+(\tau^+)e^{-t/\tau^+} \mathrm{d}\tau^+, \tag{11}$$

are true. From Eq. 11, since the integrands must match, we get

$$X^+(\tau^+) \equiv \frac{\Xi^+(\tau^+)}{\tau^+} = \sigma^+_{\text{se}}\mathcal{F}\left(\tau^+; \tau^+_{\text{se}}, \beta\right). \tag{12}$$

Validity of Eq. 10 is easily verified. From Eqs. 1 and 3, since $\mathcal{H}$ and $\mathcal{F}$ are probability distributions by definition, we have

$$\int_0^\infty \mathcal{H}\left(\xi; \tau_{\text{se}}, \beta\right) \mathrm{d}\xi = 1, \tag{13a}$$

$$\int_0^\infty \mathcal{F}\left(\tau; \tau_{\text{se}}, \beta\right) \mathrm{d}\tau = 1. \tag{13b}$$

Using Eq. 12, we therefore get

$$\int_0^\infty X^+(\tau^+)\mathrm{d}\tau^+ = \int_0^\infty \sigma^+_{\text{se}}\mathcal{F}\left(\tau^+; \tau^+_{\text{se}}, \beta\right) \mathrm{d}\tau^+, \tag{14a}$$

$$= \sigma^+_{\text{se}}\int_0^\infty \mathcal{F}\left(\tau^+; \tau^+_{\text{se}}, \beta\right) \mathrm{d}\tau^+, \tag{14b}$$

$$= \sigma^+_{\text{se}}. \tag{14c}$$

Since $\Xi(\tau) \equiv \tau X(\tau)$, we also get

$$\int_0^\infty \Xi^+(\tau^+)\mathrm{d}\ln\tau^+ = \sigma_{\mathrm{se}}^+. \tag{15}$$

By analogy, the same can be shown to be true for step up in shear, which gives us

$$X^-(\tau^-) \equiv \frac{\Xi^-(\tau^-)}{\tau^-} = \sigma_{\mathrm{se}}^-\mathcal{F}\left(\tau^-;\tau_{\mathrm{se}}^-,\beta\right), \tag{16a}$$

$$\int_0^\infty X^-(\tau^-)\mathrm{d}\tau^- \equiv \int_0^\infty \Xi^-(\tau^-)\mathrm{d}\ln\tau^- = \sigma_{\mathrm{se}}^-. \tag{16b}$$

The continuous distribution for the stretched exponential is therefore

$$X(\tau) = \sigma_{\mathrm{se}}\mathcal{F}(\tau;\tau_{\mathrm{se}},\beta) = \sigma_{\mathrm{se}}\frac{1}{\pi}\frac{\tau_{\mathrm{se}}}{\tau^2}\int_0^\infty e^{-u^\beta\cos(\pi\beta/2)}\cos\left[\frac{\tau_{\mathrm{se}}}{\tau}u - u^\beta\sin\left(\frac{\pi\beta}{2}\right)\right]\mathrm{d}u, \tag{17a}$$

$$\Xi(\tau) = \tau\sigma_{\mathrm{se}}\mathcal{F}(\tau;\tau_{\mathrm{se}},\beta) = \sigma_{\mathrm{se}}\frac{1}{\pi}\frac{\tau_{\mathrm{se}}}{\tau}\int_0^\infty e^{-u^\beta\cos(\pi\beta/2)}\cos\left[\frac{\tau_{\mathrm{se}}}{\tau}u - u^\beta\sin\left(\frac{\pi\beta}{2}\right)\right]\mathrm{d}u, \tag{17b}$$

such that

$$\sigma^+(t) = \sigma_0 + \sigma_{\mathrm{se}}^+\left[1 - e^{-\left(t/\tau_{\mathrm{se}}^+\right)^\beta}\right] = \sigma_0 + \int_0^\infty \Xi^+(\tau^+)\left(1 - e^{-t/\tau^+}\right)\mathrm{d}\ln\tau^+, \tag{18a}$$

$$\sigma^-(t) = \sigma_{\mathrm{ss}} + \sigma_{\mathrm{se}}^- e^{-\left(t/\tau_{\mathrm{se}}^-\right)^\beta} = \sigma_{\mathrm{ss}} + \int_0^\infty \Xi^-(\tau^-)e^{-t/\tau^-}\mathrm{d}\ln\tau^-. \tag{18b}$$

$\Xi(\tau)$ as obtained above can thus be co-plotted with the discrete spectrum $\sigma_i(\tau_i)$.

# 2 Fit parameters for stretched exponential fits

We list the parameters obtained for the stretched exponential fits for all the step shear rate data with Laponite shown in the paper. The fit equations used for fitting step rate data are

$$\sigma^+(t) = \sigma_0 + \sigma_{\mathrm{se}}^+\left[1 - e^{-\left(t/\tau_{\mathrm{se}}^+\right)^\beta}\right], \tag{19a}$$

$$\sigma^-(t) = \sigma_{\mathrm{ss}} + \sigma_{\mathrm{se}}^- e^{-\left(t/\tau_{\mathrm{se}}^-\right)^\beta}, \tag{19b}$$

where $\sigma(t)$ is the transient stress data in step rate tests, $\sigma_0$ is the stress at $t = 0$ in step down tests, while $\sigma_{\mathrm{ss}}$ is the steady state stress in step up tests; $\sigma_{\mathrm{se}}$ is the amount of stress change, $\tau_{\mathrm{se}}$ is the characteristic time constant of the stretched exponential function, and $\beta$ is the stretching exponent. For step down tests, $\dot\gamma_{\mathrm{i}} = 5\ \mathrm{s}^{-1}$ for all data, while $\dot\gamma_{\mathrm{i}} = 0.1\ \mathrm{s}^{-1}$ for step up tests.

Table 1: Parameters obtained for the stretched exponential fits for all the step down data shown in the paper, for Laponite.

| $\dot\gamma_{\mathrm{f}}$ [$\mathrm{s}^{-1}$] | $\sigma_0$ [Pa] | $\sigma_{\mathrm{se}}^+$ [Pa] | $\tau_{\mathrm{se}}^+$ [s] | $\beta$ [−] |
|---|---|---|---|---|
| 0.25 | 64.11 | 48.56 | 3.51 | 0.59 |
| 0.50 | 71.09 | 43.89 | 2.31 | 0.49 |
| 1.00 | 75.73 | 42.21 | 1.14 | 0.36 |
| 2.50 | 99.96 | 21.29 | 0.64 | 0.35 |

Table 2: Parameters obtained for the stretched exponential fits for all the step up data shown in the paper, for Laponite.

| $\dot{\gamma}_{\rm f}$ [s$^{-1}$] | $\sigma_{\rm ss}$ [Pa] | $\sigma_{\rm se}^{-}$ [Pa] | $\tau_{\rm se}^{-}$ [s] | $\beta$ [−] |
|---|---|---|---|---|
| 0.50 | 89.42 | 35.91 | 0.16 | 0.38 |
| 1.00 | 96.56 | 43.26 | 0.32 | 0.37 |
| 2.50 | 103.75 | 72.97 | 0.43 | 0.33 |
| 5.00 | 108.52 | 121.82 | 0.47 | 0.31 |

We also list the parameters obtained for the stretched exponential fits for all the step down in rate data with carbon black, fumed silica, and Carbopol shown in the paper.

Table 3: Parameters obtained for the stretched exponential fits for all the step down data shown in the paper, for carbon black.

| $\dot{\gamma}_{\rm f}$ [s$^{-1}$] | $\sigma_0$ [Pa] | $\sigma_{\rm se}^{+}$ [Pa] | $\tau_{\rm se}^{+}$ [s] | $\beta$ [−] |
|---|---|---|---|---|
| 0.25 | 2.25 | 11.83 | 5.46 | 0.86 |
| 0.50 | 4.95 | 11.61 | 2.99 | 0.81 |
| 1.00 | 8.2 | 11.46 | 1.48 | 0.63 |
| 2.50 | 21.76 | 8.48 | 0.48 | 0.44 |

Table 4: Parameters obtained for the stretched exponential fits for all the step down data shown in the paper, for fumed silica.

| $\dot{\gamma}_{\rm f}$ [s$^{-1}$] | $\sigma_0$ [Pa] | $\sigma_{\rm se}^{+}$ [Pa] | $\tau_{\rm se}^{+}$ [s] | $\beta$ [−] |
|---|---|---|---|---|
| 0.25 | 0.27 | 11.44 | 5.62 | 0.83 |
| 0.50 | 1.44 | 12.70 | 1.46 | 0.58 |
| 1.00 | 4.38 | 11.01 | 0.75 | 0.56 |
| 2.50 | 11.41 | 7.60 | 0.27 | 0.45 |

Table 5: Parameters obtained for the stretched exponential fits for all the step down data shown in the paper, for Carbopol.

| $\dot{\gamma}_{\rm f}$ [s$^{-1}$] | $\sigma_0$ [Pa] | $\sigma_{\rm se}^{+}$ [Pa] | $\tau_{\rm se}^{+}$ [s] | $\beta$ [−] |
|---|---|---|---|---|
| 0.25 | 52.22 | 54.55 | 0.16 | 0.28 |
| 0.50 | 70.82 | 43.37 | 0.10 | 0.28 |
| 1.00 | 82.81 | 41.97 | 0.03 | 0.25 |
| 2.50 | 129.59 | 13.72 | 0.04 | 0.31 |

# 3 Simplest thixotropic viscoplastic constitutive model

The simplest thixotropic constitutive equation based on structural kinetics was proposed by Goodeve [3] and later Moore [4]. More recent reviews have summarized this model, based on the Bingham viscoplastic model [5, 6]

$$\sigma = \sigma_{\rm y}(\lambda) + \eta(\lambda)\dot{\gamma}, \tag{20}$$

where the yield stress $\sigma_{\rm y}$ and plastic viscosity $\eta$ are functions of a structure parameter $\lambda$, each an explicit, linear function of $\lambda$, given by

$$\sigma_{\rm y}(\lambda) = \sigma_{\rm y0}\lambda, \tag{21a}$$

$$\eta(\lambda) = \eta_0\lambda, \tag{21b}$$

and this constitutes the simplest structure kinetics thixotropic constitutive equation. The structure parameter evolves via its own kinetic equation, which in its simplest form is [5, 6]

$$\frac{\mathrm{d}\lambda}{\mathrm{d}t} = k_\mathrm{A}\left(1-\lambda\right) - k_\mathrm{D}|\dot{\gamma}|\lambda, \tag{22}$$

where $k_\mathrm{A}$ and $k_\mathrm{D}$ are aggregation and destruction rate constants respectively. Solving this for step down in rate with $\dot{\gamma} = \dot{\gamma}_\mathrm{f}$, we get

$$\lambda(t) = \lambda_0 e^{-t/\tau_\lambda} + k_\mathrm{A}\tau_\lambda\left(1 - e^{-t/\tau_\lambda}\right), \tag{23}$$

where $\lambda_0$ is the initial structure parameter at the beginning of the $\dot{\gamma}_\mathrm{f}$ step, and $\tau_\lambda$ is the thixotropic timescale of change, given by

$$\tau_\lambda \equiv \frac{1}{k_\mathrm{A} + k_\mathrm{D}|\dot{\gamma}_\mathrm{f}|}. \tag{24}$$

The structure parameter at steady state is

$$\lim_{t\to\infty}\lambda(t) = \lambda_\infty = \frac{k_\mathrm{A}}{k_\mathrm{A} + k_\mathrm{D}|\dot{\gamma}_\mathrm{f}|}, \tag{25}$$

and the steady state stress is obtained from this as

$$\lim_{t\to\infty}\sigma(t) = \sigma_\infty = \frac{k_\mathrm{A}}{k_\mathrm{A} + k_\mathrm{D}|\dot{\gamma}_\mathrm{f}|}\left(\sigma_{\mathrm{y}0} + \eta_0\dot{\gamma}_\mathrm{f}\right), \tag{26}$$

The amount of structure change is obtained as $t \to \infty$, given by

$$\Delta\lambda \equiv \lambda_\infty - \lambda_0, \tag{27a}$$

$$\implies \Delta\lambda = \frac{k_\mathrm{A}}{k_\mathrm{A} + k_\mathrm{D}|\dot{\gamma}_\mathrm{f}|} - \lambda_0. \tag{27b}$$

This gives the amount of stress change due to thixotropic recovery to be

$$\Delta\sigma = \left(\sigma_{\mathrm{y}0} + \eta_0\dot{\gamma}_\mathrm{f}\right)\Delta\lambda, \tag{28a}$$

$$\implies \Delta\sigma = \left(\sigma_{\mathrm{y}0} + \eta_0\dot{\gamma}_\mathrm{f}\right)\left(\frac{k_\mathrm{A}}{k_\mathrm{A} + k_\mathrm{D}|\dot{\gamma}_\mathrm{f}|} - \lambda_0\right). \tag{28b}$$

We can see that $\tau_\lambda$ increases as $\dot{\gamma}_\mathrm{f}$ decreases, for a given material ($k_\mathrm{A}$ and $k_\mathrm{D}$ fixed). This is the same trend that we observe in the paper for $\tau_1^+$ with $\dot{\gamma}_\mathrm{f}$. The most extreme case of thixotropy is when the final shear rate vanishes, such that

$$\lim_{\dot{\gamma}_\mathrm{f}\to 0}\tau_\lambda \equiv \lim_{\dot{\gamma}_\mathrm{f}\to 0}\frac{1}{k_\mathrm{A} + k_\mathrm{D}|\dot{\gamma}_\mathrm{f}|} = \frac{1}{k_\mathrm{A}}, \tag{29}$$

and this gives the longest timescale of recovery. The largest amount of relative stress recovered is also obtained as the final shear rate vanishes, such that

$$\lim_{\dot{\gamma}_\mathrm{f}\to 0}\frac{\Delta\sigma}{\sigma_\infty} = 1 - \lambda_0, \tag{30}$$

and corroborates with results in the paper.

# References


[1] M. N. Berberan-Santos, E. N. Bodunov, and B. Valeur. Mathematical functions for the analysis of luminescence decays with underlying distributions 1. Kohlrausch decay function (stretched exponen-

tial). *J. Chem. Phys.*, 315:171–182, 2005.

[2] D. C. Johnston. Stretched exponential relaxation arising from a continuous sum of exponential decays. *Phys. Rev. B*, 74:184430, 2006.

[3] C. Goodeve and G. Whitfield. The measurement of thixotropy in absolute units. *Trans. Faraday Soc.*, 34:511–520, 1938.

[4] F. Moore. The rheology of ceramic slips and bodies. *Trans. Br. Ceram. Soc.*, 58:470–494, 1959.

[5] J. Mewis and N. J. Wagner. Thixotropy. *Adv. Colloid Interface Sci.*, 147–148:214–227, 2009.

[6] R. G. Larson and Y. Wei. A review of thixotropy and its rheological modeling. *J. Rheol.*, 63(3): 477–501, 2019.
